# Supplementary material for: ScientistOne: Towards Human-Level Autonomous Research via Chain-of-Evidence
Source: arXiv:2605.26340 source file (2026-05-25)
Supplement: Supplementary file 1 [file 012_appendix-archived.tex]

%% ============================================================
%% Appendix
%% ============================================================

\section{CoE Audit: Sub-Code Definitions}
\label{app:subcodes}

\todo{Full sub-code tables for each integrity check. These provide the rubric for reproducibility.}

\subsection{Score Verification Failure Codes}

\begin{table}[h]
\centering
\small
\begin{tabular}{@{}clp{7cm}@{}}
\toprule
\textbf{Code} & \textbf{Label} & \textbf{Description} \\
\midrule
SF-1 & Genuine discrepancy & Paper score differs from evaluator rerun mean beyond adaptive tolerance, with consistent metric and scale \\
SF-2 & Metric mismatch & Paper and evaluator report different metrics or scales (e.g., percentage vs.\ fraction, inverted objective) \\
SF-3 & Metric inversion & Paper score is the reciprocal of the evaluator score, suggesting an inverted optimization direction \\
SF-4 & Evaluator failure & All $N{=}3$ evaluator reruns crashed or returned null \\
SF-5 & Evaluator timeout & All $N{=}3$ evaluator reruns exceeded the time limit \\
SF-6 & Score extraction failure & No headline score could be extracted from the agent's logs or paper \\
\bottomrule
\end{tabular}
\end{table}


\subsection{Hack Verification Sub-Codes}

\begin{table}[h]
\centering
\small
\begin{tabular}{@{}clp{7cm}@{}}
\toprule
\textbf{Code} & \textbf{Label} & \textbf{Description} \\
\midrule
RWH-1 & Evaluator tampering & Solver modifies evaluator code, data files, or scoring logic \\
RWH-2 & Trivial solution & Solver returns a hardcoded or degenerate answer that exploits evaluator edge cases \\
RWH-3 & Score gaming & Solver optimizes a proxy that inflates the score without solving the underlying problem \\
RWH-4 & Data leakage & Solver reads test data or evaluation labels at training time \\
RWH-5 & Specification exploit & Solver exploits an unintended loophole in the task specification (e.g., column permutation in LLM-SQL) \\
\bottomrule
\end{tabular}
\end{table}


\subsection{Reference Verification Sub-Codes}

\begin{table}[h]
\centering
\small
\begin{tabular}{@{}clp{7cm}@{}}
\toprule
\textbf{Code} & \textbf{Label} & \textbf{Description} \\
\midrule
RF-1 & Hallucinated reference & Reference does not exist anywhere (Scholar, DBLP, arXiv) \\
RF-2 & Memory-recalled reference & Reference is real but recalled from model weights, not retrieved; metadata often corrupted \\
\bottomrule
\end{tabular}
\end{table}


\subsection{Method-Code Alignment Sub-Codes}

\begin{table}[h]
\centering
\small
\begin{tabular}{@{}clp{7cm}@{}}
\toprule
\textbf{Code} & \textbf{Label} & \textbf{Description} \\
\midrule
MCA-0 & Aligned & Paper accurately reflects implemented code \\
MCA-1 & Embellished & Paper adds sophistication not in the code \\
MCA-2 & Wrong method & Paper describes a fundamentally different algorithm \\
MCA-3 & Orphan description & Method described but code never ran or crashed \\
\bottomrule
\end{tabular}
\end{table}


\section{Per-Paper CoE Audit Results}
\label{app:per_paper}

\todo{Full per-paper results for all N papers. One row per (system, seed, task) with all check results + forensic CPR. This is the evidence backing the main integrity table.}

\todo{Consider: format as a large table, or as structured JSON/CSV in supplementary materials?}


\section{Solver Score Details}
\label{app:solver_details}

\todo{ADRS v2 normalization explanation.
Per-seed solver scores for all systems (not just the aggregate in the main table).
For AI2Scientist: which config was used per task? Link to ablation data.}


\section{System Implementation Details}
\label{app:system_details}

\subsection{Solver Architecture}

The Solver consists of two agents.
The \emph{Solution Development Agent} receives an idea and task-specific instructions, operates in a sandboxed environment with tools for file I/O, command-line execution, solution management, and knowledge base retrieval, and follows an iterative refinement loop---executing experiments, debugging errors, and optimizing validation metrics---while maintaining an experimental log.
The \emph{Report Writing Agent} parses experimental artifacts to generate a technical report summarizing methodology and outcomes.

\subsection{Ablation Study}

Following PEE, the system selects the global best solution for further validation.
An ablation agent identifies the solution's core components and proposes controlled experiments to isolate their contributions.
These ablated versions are implemented and re-evaluated to quantify the performance impact of specific architectural or algorithmic choices.

\subsection{Claim Verifier: Per-Type Verification Rules}
\label{app:claim_verifier_rules}

The Claim Verifier dispatches on the four claim types defined in \cref{sec:coe}.
The writer commits each claim's evidence via annotation tags---a line in the experimental log, a citation key, an internal ablation, a baseline from the PI brief, or an explicit ``unsourced'' marker---and the verifier maps that evidence onto the claim type's verification rule:

\begin{itemize}\itemsep2pt \parskip0pt
  \item \textbf{Numerical claims} are checked by numeric tolerance against the cited evidence (log line, ablation entry, or PI baseline), with a $\pm 3$-line window on log lines and unit-aware normalizations for percent-versus-fraction and millisecond-versus-second drift.
  \item \textbf{Citation claims} are checked by resolving the cite key against the bibliography and then asking a one-shot LLM judge (JSON mode) whether the cited work's abstract supports the specific assertion.
  \item \textbf{Methodological claims} are checked by substantive textual overlap against the cited region of the experimental log.
  \item \textbf{Conclusion claims} are detected post-hoc by scanning for comparison language, linked to supporting numerical claims by token and number overlap, and---when parseable---validated by arithmetic check against pairwise differences.
\end{itemize}

\noindent Claims tagged ``unsourced'' or carrying malformed annotations are dropped automatically; each records a break code for downstream reporting.

\subsection{Claim-Evidence Graph Format}

For every annotation the verifier emits one record: a claim id, a type tag, the section it appears in, the rendered sentence text, a structured value where recoverable, and an ordered evidence chain whose links each carry a source URI, content hash, extracted text, verification method, and pass/partial/fail status.
A verification summary attaches the appropriate break code when the chain is broken, distinguishing the failure modes catalogued in \cref{tab:coeaudit_checks}.
The sidecar \texttt{corrections.json} records the same failures in a form the Refiner consumes, so a failed chain produces both a diagnostic in the CEG and a directed edit on the draft.

\subsection{Paper Writer: GROUND and CRITIC Details}

\textsc{Ground} runs deterministic checks: the published score is present, baselines are labelled \textsc{verified} or \textsc{estimated} (unattributed ``leaderboard'' references are flagged), every referenced file exists, all sections are present, and hyperbole and known score mismatches are accounted for.
\textsc{Critic} is one LLM call that audits story-level coherence (gap--approach alignment, contradictions, overclaims, missing comparisons, baseline fairness, honest limitations) and returns \textsc{pass} or a list of \textsc{major}/\textsc{minor} issues.
\textsc{Resolve} rewrites the representation against both lists in one call.
The loop terminates on convergence (zero flags) or plateau (the flag count stops decreasing), and a final grounding ratio below a configured threshold raises a hard error.


\section{CoE Audit Procedure and Reproducibility}
\label{app:audit_implementation}

\coeaudit{} is designed for reproducibility.
\Cref{tab:audit_procedure} summarizes the automation level of each component.
Score Verification, Hack Verification, and the forensic CPR evidence-matching step are fully deterministic---they use evaluator re-runs, checksums, regex, and numeric comparison with no LLM involvement.
Reference Verification is primarily API-based (Semantic Scholar lookup), with an LLM disambiguation step for title-only matches.
Method-Code Alignment and forensic CPR claim extraction are LLM-judged.

\begin{table}[h]
\centering
\small
\caption{\coeaudit{} automation level per component.}
\label{tab:audit_procedure}
\begin{tabular}{@{}lll@{}}
\toprule
\textbf{Component} & \textbf{Automation} & \textbf{Model (if LLM)} \\
\midrule
Score Verification & Fully automated & --- \\
Hack Verif.\ & Fully automated & --- \\
Reference Verification & Automated + LLM disambiguation & Gemini~3.0 Flash \\
Method-Code Alignment & LLM-judged & Gemini~3.1 Pro \\
Forensic CPR (extraction) & LLM-judged & Gemini~3.0 Flash \\
Forensic CPR (matching) & Fully automated & --- \\
\bottomrule
\end{tabular}
\end{table}

The full pipeline runs unattended.
\todo{Report: time per paper (approx), total cost for the 75-paper audit, and whether results are deterministic across runs for the automated components.}

\subsection{Claim Provenance Rate: Forensic Extraction}
\label{app:forensic_cpr}

Forensic \cpr{} is computed post-hoc from released artifacts in three stages:

\begin{enumerate}[nosep,leftmargin=*]
  \item \textbf{Claim extraction.} An LLM classifier (Gemini~3.0 Flash) reads each sentence and labels it as a numerical result claim, a non-result sentence, or ambiguous. Only numerical result claims enter the verification pool.
  \item \textbf{Evidence matching.} Each claim is matched against execution logs via metric-name co-occurrence: we check whether the metric name in the claim appears in a log line containing a numeric value within 1\% tolerance. A guarded value-only fallback handles absent metric names.
  \item \textbf{Verification.} A claim is verified if a matching log line is found. Per-paper forensic $\text{CPR}_{\text{numerical}}$ is the fraction of extracted claims that are verified.
\end{enumerate}

Native \cpr{} is computed from provenance annotations emitted by the system at production time.
Each claim in \texttt{claims.jsonl} carries a verification status (\texttt{passed}, \texttt{partial}, or \texttt{failed}) from the Claim Verifier.
Only \sys{} produces native \cpr{}.

\subsection{Implementation Details}

\todo{Detailed description of each check's implementation:
- Score Verification: evaluator re-run procedure, adapter per system, tolerance, failure classification
- Hack Verification: evaluator checksum comparison, score consistency threshold
- Reference Verification: S2 API querying, DOI/arXiv/title lookup, similarity threshold
- Method-Code Alignment: LLM prompt, model, scoring rubric
- Forensic CPR: claim extraction prompt, metric-name matching algorithm, trivial value filter
This enables reproducibility and addresses the "self-graded" concern.}


\section{\sys{} Native CPR}
\label{app:native_cpr}

\todo{Per-type CPR breakdown for \sys{} papers:
- CPR\_numerical
- CPR\_citation
- CPR\_methodological
- CPR\_conclusion (if implemented)
With example evidence chains for each type.}


\section{Problem Investigator Details}
\label{app:pi_details}

\todo{PI pipeline details that don't fit in the main paper:
- Number of PDFs read per topic
- Quality gate criteria and pass rate
- Example PI brief structure
- PI ablation results (does PI context help solver? Help paper quality?)}


\section{MLE-Bench and Parameter Golf Evaluation}
\label{app:mle-pg-eval}
